# Supplementary material for: Evolutionary Hierarchical Harvest Schedule Optimization for Food Waste Prevention
Source: arXiv:2112.10712 source file (2021-12-20)
Supplement: Supplementary file 1 [file supplementary.tex]

\section{Supplementary Material}

\subsection{Detailed Description of the Dataset}
The given dataset was distributed by Syngenta within the scope of the Crop Challenge\footnote{\url{https://www.ideaconnection.com/syngenta-crop-challenge/}} 2021 and contains daily GDU time series from 01/01/2009 to 12/31/2019 for two sites (named as site 0 and site 1). Original, earliest, and latest planting dates of 2569 crop species (\num{1375} for site 0, \num{1194} for site 1) and the required GDUs for each of those are given. On this dataset, two scenarios are exercised with randomly drawn desired harvest quantities per species. They are sampled from Gaussian distributions $\mathcal{N}(\mu,\sigma)$ with $\mathcal{N}(250,100)$ and $\mathcal{N}(350,150)$, respectively. For scenarios S1, the sites have weekly harvest capacity limits (7000 units for site 0, 6000 units for site 1) whereas for S2, the capacity is not given. The optimization is performed for harvest season 2020/2021.

Plant and harvest windows for each plant species and both sites are shown in Figure~\ref{fig:plant_harvest_dist} colored in blue and orange, respectively, in the upper plots. For site 1, they are quite continuous but for site 0, one can see accumulations regarding possible planting days around February and May. As a result, one can see two accumulations for the harvest days around November and the following February. The plant and harvest day distribution for site 1 is considerably smoother, although accumulations can also be seen here. A deliberate choice of the individual yield per plant could equalize this effect. However, yields are roughly drawn from Gaussian distributions in our case. The lower plots in Figure~\ref{fig:plant_harvest_dist} confirm that by showing that weighting the day distribution by corresponding yield per species is not flattening the overall shape\textemdash neither for scenario S1 nor for S2.
\begin{figure}[t]
	\centering
	\includegraphics[width=0.9\columnwidth]{images/plant_harvest_dist.pdf}
	\caption{Distribution of possible plant and harvest days for all species and both sites. The upper plots show the spans (windows) of possible plant and harvest days for each plant species. The middle plots show the absolute abundance (frequency) of the respective days by summation over all species for the respective site. Additionally, the lower plots show the harvest day abundance weighted with the harvest yield for both scenarios of the corresponding species by multiplication.}
	\label{fig:plant_harvest_dist}
\end{figure}

\subsection{GDU Accumulation Forecast with GPR Model}
A naive approach to forecast the GDU accumulation would be to group the historical data by calendar date\textemdash i.e. month and day\textemdash and average over years. One would get an estimate for the daily jitter (or noise) by additional calculation of the standard deviation. Finally, the forecast could be a sampling of the future calendar days by a Gaussian distribution with the calculated means and standard deviations. However, this ansatz has some disadvantages. On the one hand, we have a problem when it comes to leap years. There is no clear assignment of \enquote{leap-year days} to \enquote{non-leap-year days}. However, this effect has not a severe impact, which is why we would just drop the leap days from the dataset. A more important drawback, on the other hand, is that this method is blind for possible underlying seasonalities or trends. This gets obvious if you think about trends due to climate change or seasonalities beyond annual scale, as\textemdash for instance\textemdash the El Niño phenomenon. Averaging over years would make those effects invisible or only noticeable by an increase of the standard deviations. This is, why we prefer to forecast the GDU accumulation by using a GPR model.

GPR models use kernels as priors for data prediction, \mbox{inter-,} and extrapolation. If we choose those kernels deliberately, we can include our knowledge about seasonality into the GPR process. We will choose a kernel that is a sum over the following fundamental kernels:
\begin{itemize}
	\item a periodic exponential kernel with annual periodicity to represent the obvious annual seasonality,
	\item a linear kernel to represent possible large-scale trends over the historic period (for instance climate change),
	\item a bias kernel to cope with the fact that the GDU values are not centered around zero, and
	\item a white noise kernel to estimate random daily temperature fluctuations.
\end{itemize}

The forecast results for the GDU accumulation functions are shown in Figure~\ref{fig:gdu_pred} for both sites. Although there are some anomalies at some days, one cannot see any other periodic behavior in the residue plots in the two figures that would not have been caught by the GPR model. Thus, we can state that the GPR model covers the given dataset quite well. Due to the periodicity, we can simply extrapolate into the future (i.e. $d\geq 0$). The result for both sites is shown in Figure~\ref{fig:gdu_forecast}. All in all, the GDU data of site 1 has a higher volatility than site 0 which is reflected in the overall higher standard deviation compared to site 0.

\begin{figure}[ht]
	\centering
	\includegraphics[width=0.9\columnwidth]{images/GDU_GP_pred_site0.pdf}
	\includegraphics[width=0.9\columnwidth]{images/GDU_GP_pred_site1.pdf}
	\caption{GPR prediction result for site 0 and 1. In order to get a more compact optimization domain, the day indices are normalized to years. In the upper plot, the data is shown as well as the mean prediction result and the confidence band with represents $\pm 2 \sigma$ in terms of Gaussian standard deviation. The lower plot shows the residues with respect to mean with the standard deviation of prediction as error bars.}
	\label{fig:gdu_pred}
\end{figure}

\subsection{Harvest Schedule Results for Site 0}
Figures~\ref{fig:loss_hist_s1_site0} shows the optimization process for S1 and site 0. The optimization results for all 3 scenarios are shown in Figure~\ref{fig:harvest_results_site0}.

\begin{figure}[t]
	\centering
	\includegraphics[width=0.9\columnwidth]{images/loss_hist_site0_sc1.pdf}
	\caption{Optimization process for scenario S1 and site 0. The different colors represent 3 independent runs. The two lower plots show the components of the loss vector $L_+$ and $L_-$ against number of iterations. The upper plot shows the mutation rate for each successful improvement as a dot.}
	\label{fig:loss_hist_s1_site0}
\end{figure}
\begin{figure}[ht]
	\centering
	    \includegraphics[width=0.9\columnwidth]{images/harvest_site0_sc1_run02.pdf}
	    \includegraphics[width=0.9\columnwidth]{images/harvest_site0_sc2_run01.pdf}
    	\includegraphics[width=0.9\columnwidth]{images/harvest_site0_sc3_run02.pdf}
	\caption{Weekly harvest quantity for all 3 scenarios on site 0. The orange bars symbolize the harvest per week for an unoptimized schedule given in the dataset. Blue bars show our optimization result. The dashed lines mark $C_\text{target}$ (red) and $C_\text{need}$ (purple). For the uncertainty estimation, plotted as error bars, \num{100} harvest matrices are drawn from the GPR model for the GDU accumulation functions.}
	\label{fig:harvest_results_site0}
\end{figure}

\subsection{Cyclic harvest weeks}
In addition to a single harvest time window, it is possible to define a day-to-week mapping for a cyclic harvest season $\mathbf{W}_\text{cyclic}~\in~\{0;1\}^{|\mathcal{D}|\times 52}$ by
\begin{align}
    \begin{aligned}
       \mathbf{W}_\text{cyclic} &= \{W_\text{cyclic}(i,j)\},\\
       &W_\text{cyclic}(i,j) =
        \begin{cases}
        1 & \lfloor \frac{i+\delta}{7}\rfloor\bmod{52} = j\\
        0 & \text{otherwise}
        \end{cases}\,, 
    \end{aligned}
\end{align}
where the 52 arises from the number of weeks per year. This means that one considers the same seeding over multiple seasons, i.e. repeating harvest plans can also be optimized. Figure~\ref{fig:harvest_cyclic} shows an exemplary optimization result of site 1 and scenario S2-1. Especially in this case, the overshoot is reduced to below \SI{0.2}{\percent} with respect to the capacity limit. The optimization process is shown in Figure~\ref{fig:loss_hist_cyclic}.
\begin{figure}[t]
	\centering
	\includegraphics[width=0.9\columnwidth]{images/harvest_site1_sc2_cyclic_run02.pdf}
	\caption{Weekly harvest quantity for scenario S2-1 and site 1 with cyclic harvest weeks. In the legend, all benchmark values are stated (cf. Table~\ref{tab:benchmarks}). For the uncertainty estimation, plotted as error bars, \num{100} harvest matrices are drawn from the GPR model.}
	\label{fig:harvest_cyclic}
\end{figure}
\begin{figure}[t]
	\centering
	\includegraphics[width=0.9\columnwidth]{images/loss_hist_site1_sc2_cyclic.pdf}
	\caption{Optimization process for scenario S1-1 and site 1 with cyclic harvest weeks. The different colors represent 3 independent runs. The two lower plots show the components of the loss vector $L_+$ and $L_-$ against number of iterations. The upper plot shows the mutation rate for each successful improvement as a dot.}
	\label{fig:loss_hist_cyclic}
\end{figure}
